# Supplementary material for: Risk Controlled Image Retrieval
Source: arXiv:2307.07336 source file (2025-01-06)
Supplement: Supplementary file 1 [file appendix.tex]

\section{Implementations}
\subsection{Network Architectures}

Figure \ref{fig_networks} illustrates the network architectures of the three image retrieval models used in our experiments: 
\begin{itemize}
    \item The \textbf{Deterministic} model is composed of ResNet-50 \cite{he2016deep} backbone, a GeM layer \cite{radenovic2018fine}, a fully connected layer and a L2-normalization layer. The Deterministic model is trained with the triplet loss \cite{schroff2015facenet} (the loss function will be explained soon).
    \item  The \textbf{MCD} model is the same as the Deterministic except that we apply dropout to all conventional layers of the backbone during both training and testing time.
    \item  The \textbf{BTL} model has an additional variance head compared to the Deterministic model, and it is trained with the Bayesian triplet loss \cite{warburg2021bayesian} (the loss function will be explained soon).
    \item The \textbf{Deep Ensemble} is built with $5$ Deterministic models that are trained from different initial weights.

\end{itemize}

\begin{figure}[ht]
    \begin{center}
       \includegraphics[width=0.5\linewidth]{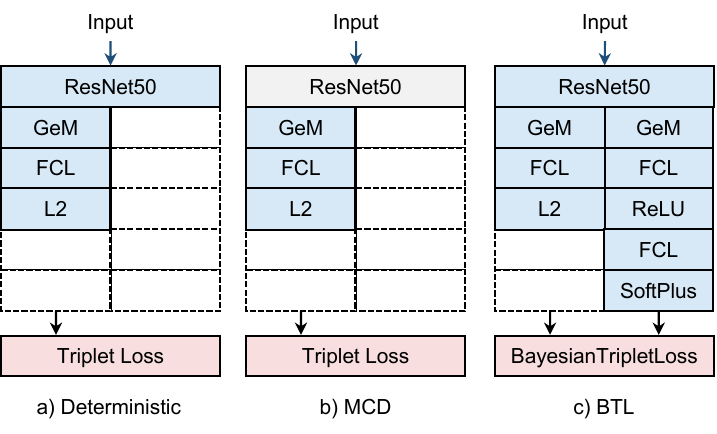}
    \end{center}
    \vspace{-0.5cm}
       \caption{The network architectures of different image retrieval models.} 
       \label{fig_networks}
 \end{figure}

\subsection{Loss Functions}
% We describe the loss functions we used to different image retrieval methods.
\subsubsection{Bayesian Triplet Loss}
Bayesian triplet loss was proposed in \cite{warburg2021bayesian}, and we include it here for completeness. In this setting, embeddings are modeled as a Gaussian distribution $\mathcal{N}(f_\phi(X), f_\sigma^2(X))$. Denote embeddings of query, positive, and negative images as $a$, $p$, and $n$, respectively. The probability that a query is closer to a positive than a negative is
\begin{equation}
    \label{eq_bayesian_triplet}
P(\Vert a - p \Vert^2 - \Vert a -n \Vert^2  < -m),
\end{equation}
where $m$ is a predefined margin. Equation (\ref{eq_bayesian_triplet}) is equivalent to 
\begin{equation}
    \label{eq_bayesian_triplet2}
    P(\tau < -m),
\end{equation} 
where $\tau=\sum_{d=1}^D\left(a_d-p_d\right)^2-\left(a_d-n_d\right)^2$, and $D$ is the dimension of the embedding. Since $\tau$ will approximate a Gaussian distribution when $D$ is large, we can obtain the leading two moments of $\tau$ as 
\begin{equation}
    \begin{aligned}
    \mu &= \mu_{p}^{2}+\sigma_{p}^{2}-\mu_{n}^{2}-\sigma_{n}^{2}-2 \mu_{a}\left(\mu_{p}-\mu_{n}\right), \\
    \sigma^2 &= 2[\sigma_{p}^{4}+2 \mu_{p}^{2} \sigma_{p}^{2}+2\left(\sigma_{a}^{2}+\mu_{a}^{2}\right)\left(\sigma_{p}^{2}+\mu_{p}^{2}\right)- 2 \mu_{a}^{2} \mu_{p}^{2}\\&-4 \mu_{a} \mu_{p} \sigma_{p}^{2}] + 2[\sigma_{n}^{4}+2 \mu_{n}^{2} \sigma_{n}^{2}+2\left(\sigma_{a}^{2}+\mu_{a}^{2}\right)\left(\sigma_{n}^{2}+\mu_{n}^{2}\right)\\&-2 \mu_{a}^{2} \mu_{n}^{2}-4 \mu_{a} \mu_{n} \sigma_{n}^{2}] -8 \mu_{p} \mu_{n} \sigma_{a}^{2}.
    \end{aligned}
\end{equation}
The loss is obtained as 
\begin{equation}
\mathcal{L}_{BTL}=-\frac{1}{T}\sum_{t=1}^T\log P(\tau < -m),
\end{equation}
where $T$ is the number of triplets in a batch.

\subsubsection{Triplet Loss}
In the triplet loss \cite{schroff2015facenet} setting, we denote embeddings of query, positive, and negative images as $a$, $p$, and $n$, respectively.
\begin{equation}
    \mathcal{L}_{TL}=\frac{1}{T}\sum_{t=1}^T\max\left(0, \Vert a - p \Vert^2 - \Vert a -n \Vert^2 + m \right),
\end{equation}
where $T$ is the number of triplets in a batch, $m$ is a predefined margin.

% \subsection*{KL-divergence Loss \cite{chang2020data}}
% The embeddings are modelled as Gaussian distributions $\mathcal{N}(f_\phi(X), f_\sigma^2(X))$.
% \begin{equation}
%     \begin{aligned}
%     \mathcal{L}_{KL}&=KL(\mathcal{N}(f_\phi(X), f_\sigma^2(X))||\mathcal{N}(0, I))\\
%     &=-\frac{1}{2}(1+\log f^2_\sigma(X)-f^2_\phi(X)-f^2_\sigma(X)).
%     \end{aligned}
% \end{equation}
% When training the DUL feature extractor and the DUL uncertainty estimator, we utilize a weight sum of the triplet loss and the KL-divergence loss, expressed as $\mathcal{L}_{total}=\mathcal{L}_{TL}+\lambda \cdot \mathcal{L}_{KL}$ and $\lambda=10^{-4}$.

When training Deterministic, MCD and BTL models, we follow \cite{warburg2021bayesian} and use online hardest mining to generate triplet tuples. Specifically, we first randomly select a query image $X_i^q$. Then, we select a positive image $X_i^p$ from the same class that has the largest embedding distance to the query image as $X_i^q$. Finally, we select a batch of negative images $\{X_{i,1}^n, X_{i,2}^n,.., X_{i, J}^n\}$ from a different class that has the smallest embedding distance to the query. We refresh the embedding cache at the beginning of every epoch.

\subsection{Metrics}
\begin{itemize}
    \item \textbf{Recall@1}: The Recall@1 is the percentage of queries whose top-$1$ retrieved sample is the true nearest neighbor of the query.
    \item \textbf{Reliability diagram}: Given finite query samples, the trained uncertainty estimator estimates the uncertainty for each query sample. These uncertainties are then normalized to fit within the range of $[0, 1.0]$ \cite{warburg2021bayesian}. We organize the query samples into $10$  bins based on their uncertainties, grouping them into intervals such as $[0, 0.1), [0.1, 0.2), .., [0.9, 1.0]$. By calculating the recall@1 for the query samples in each bin, we can evaluate how well the uncertainty estimator is calibrated. Ideally, we expect the recall@1 to decrease proportionally with the uncertainty, as depicted by the dashed line in the reliability diagram.
\end{itemize}

\begin{figure}[ht]
    \centering
    \includegraphics[width=1\columnwidth]{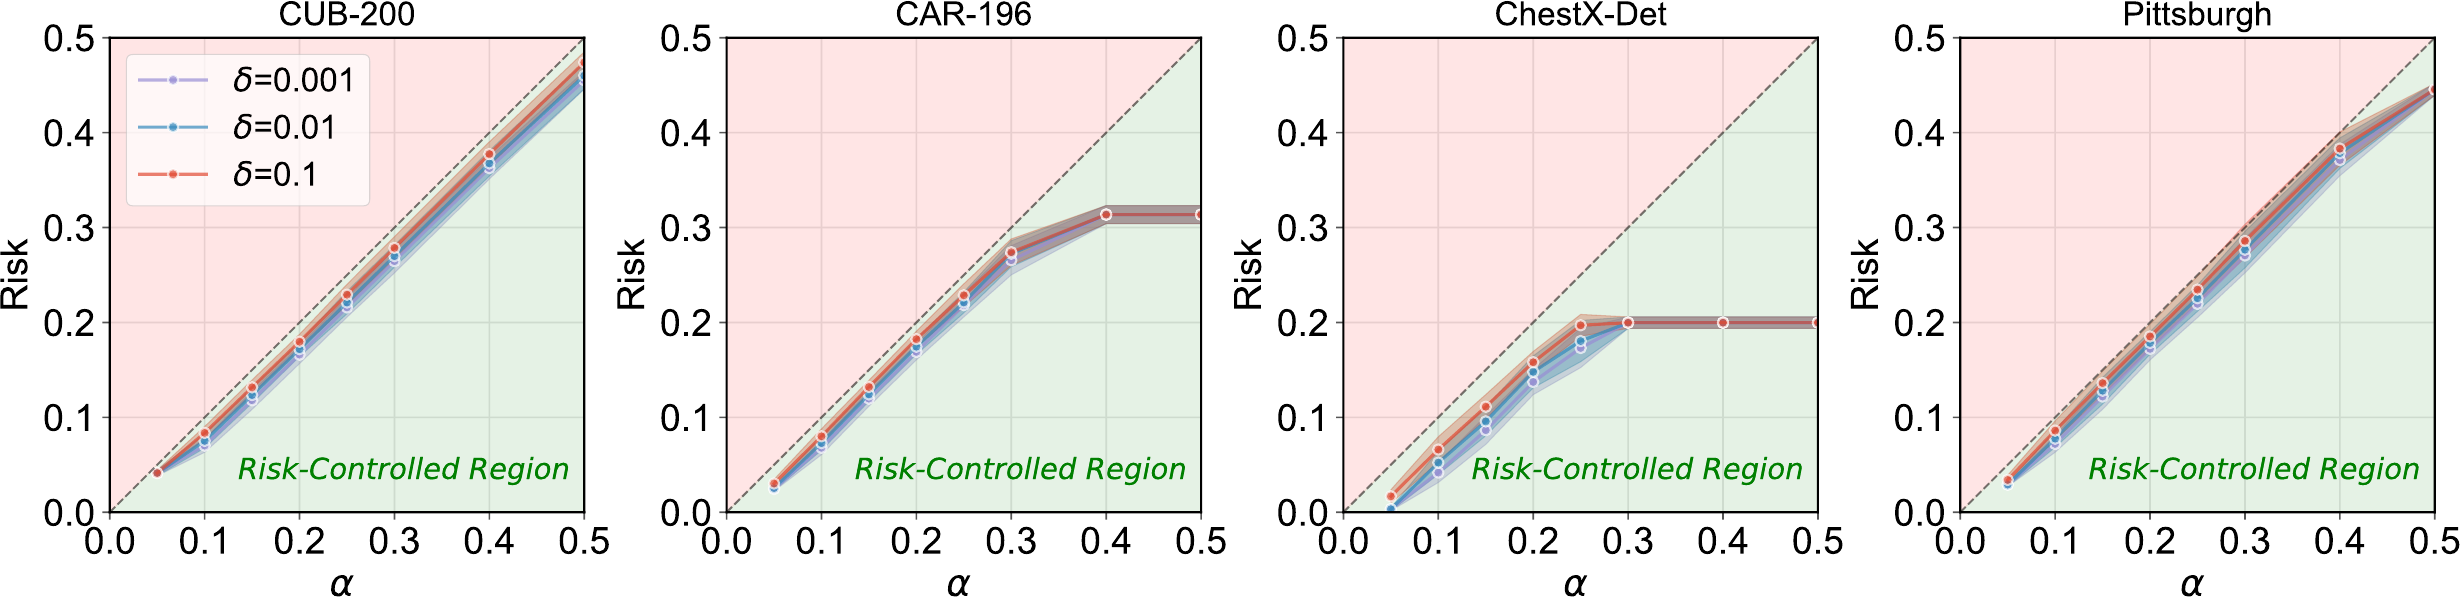} 
    \caption{The risks on different test sets with different error rates by BTL\sysr: smaller $\delta$ leads to more conservative retrievals (e.g., larger retrieval size). The colored shadows represent the standard deviation of the results of $10$ trials.}
    \label{fig_cub200_risk_control_delta}
\end{figure}

\begin{figure}[ht]
    \centering
    \includegraphics[width=1\columnwidth]{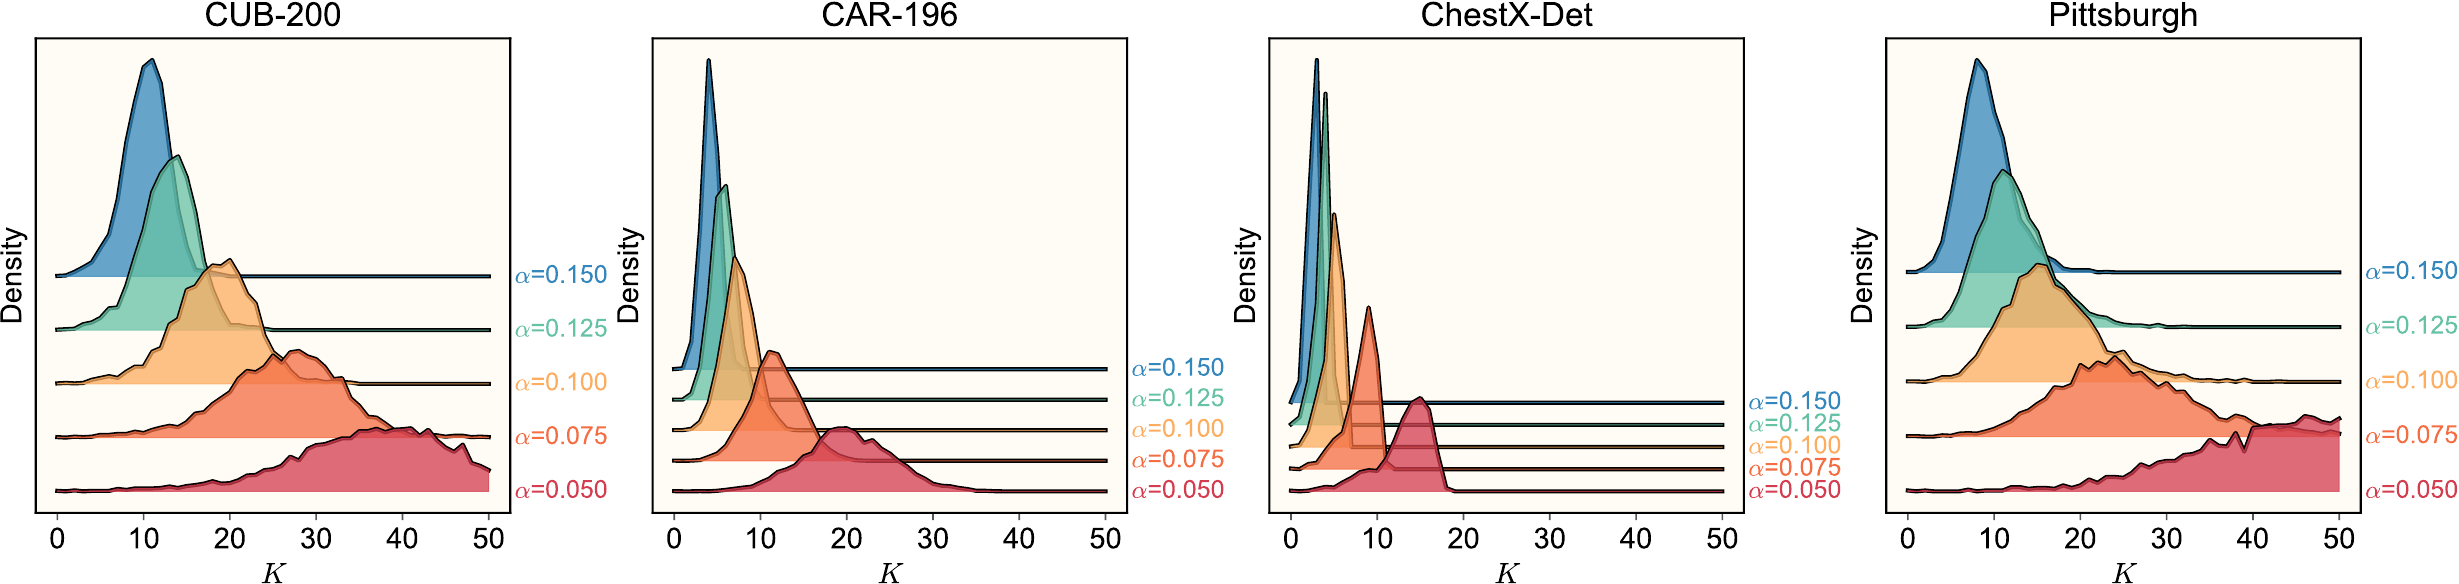} 
    \caption{The retrieval size, $K$, on different test sets by BTL\sysr: retrieval set size adapts to the risk level $\alpha$.}
    \label{fig_cub200_k_spread}
\end{figure}

\begin{figure}[!t]
    \centering
    \includegraphics[width=0.6\columnwidth]{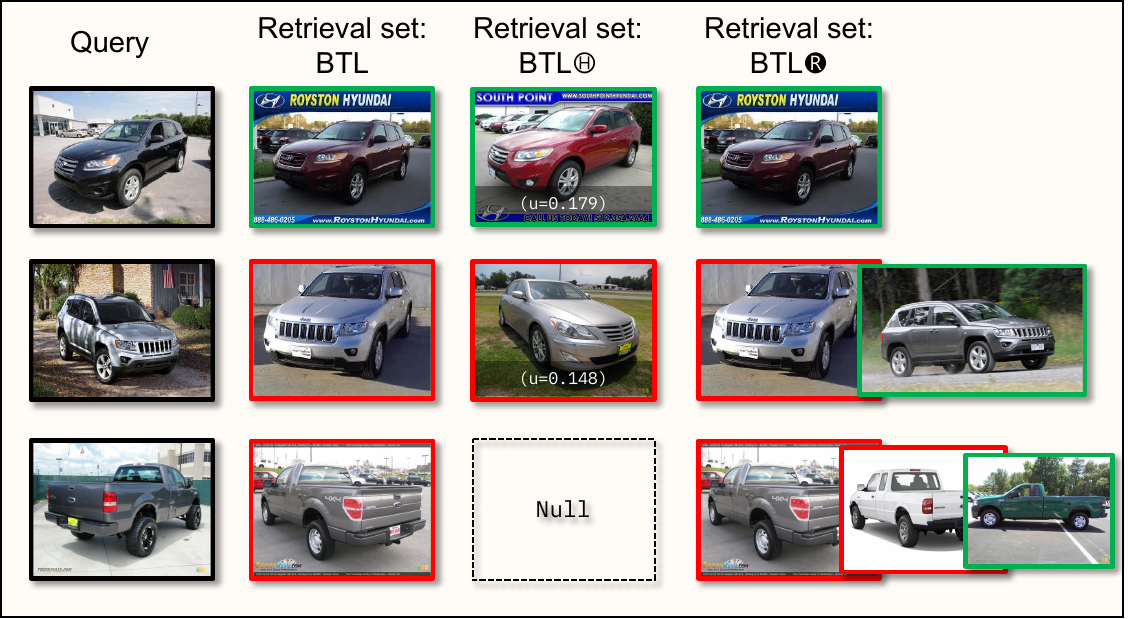} 
    \caption{The qualitative visualization of retrieval sets on the CAR-196 test set by different methods ({\textcolor{color_wrong}{Red border} \raisebox{-0.05cm}{\includegraphics[width=14pt]{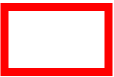}}} denotes a wrong candidate, while {\textcolor{color_correct}{green border} \raisebox{-0.05cm}{\includegraphics[width=14pt]{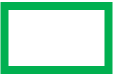}}} correct): BTL\sysr\ adjusts the size of retrievals to reflect the uncertainty while ensuring coverage ($\alpha=0.2$ and $\delta=0.1$).}
    \label{fig_qua}
\end{figure}

\section{Experimental Results}

Figure \ref{fig_cub200_risk_control_delta} shows the empirical risk with different $\delta$ on the different test sets. With a smaller $\delta$, \sysname\ would be more conservative (i.e., larger retrieval size) to ensure the risk is below the given $\alpha$. 

Figure \ref{fig_cub200_k_spread} presents the distribution of retrieval size on different test sets. It is evident that the retrieval size varies with the risk level $\alpha$: a smaller $\alpha$ results in a larger retrieval size, and vice versa. This helps end users save time on easy queries and focus on more difficult ones.

Figure \ref{fig_qua} shows the qualitative visualization of retrievals on the CAR-196 dataset by different methods. In the first row, it is evident that when a relatively easy query is provided, all methods successfully retrieve the correct results. Moving on to the second row, where the query is more challenging, the fixed-size retrieval method fails without any indication, and BTL\sysh\ fails as well with a low heuristic number. However, BTL\sysr\ takes into account the difficulty of the query and retrieves an additional candidate, resulting in the correct answer. The third row represents a more demanding query. BTL\sysh\ generates no candidate, while BTL\sysr\ retrieves more candidates to meet the coverage requirement.
